# Supplementary material for: Wav2Gloss: Generating Interlinear Glossed Text from Speech
Source: arXiv:2403.13169 source file (2024-06-06)
Supplement: Supplementary file 1 [file 02-results-by-language.tex]

\section{Results by Language}
\label{apdx:results-by-language}
See Tables \ref{tab:owsm-multi-results}, \ref{tab:wavlm-multi-results}, \ref{tab:xlsr-multi-results}, \ref{tab:owsm-single-results}, \ref{tab:wavlm-single-results}, \ref{tab:xlsr-single-results}.
\input{tables/owsm-multi-results}
\input{tables/wavlm-multi-results}
\input{tables/xlsr-multi-results}
\input{tables/owsm-single-results}
\input{tables/wavlm-single-results}
\input{tables/xlsr-single-results}
